# Supplementary material for: Transverse spin gradient functional for non-collinear spin density functional theory
Source: arXiv:1212.3658 source file (2013-09-20)
Supplement: Supplementary file 1 [file sge_functional_supplemental.pdf]

# Transverse spin gradient functional for non-collinear spin density functional theory

***Supplemental material***


F. G. Eich[1,2,*] and E. K. U. Gross[1]

[1]*Max-Planck-Institut für Mikrostrukturphysik, Weinberg 2, D-06120 Halle, Germany*

[2]*Institut für Theoretische Physik, Freie Universität Berlin, Arnimallee 14, D-14195 Berlin, Germany*



(Dated: September 1, 2013)


## CONSTRAINING FIELD FOR SPIN SPIRALS IN THE UNIFORM ELECTRON GAS

Here we demonstrate that the constraining field yielding the spin-spiral-wave (SSW) magnetization is an external magnetic field of the form

$$\boldsymbol{B}(\boldsymbol{r}) = \begin{pmatrix} A\cos(\boldsymbol{q}\cdot\boldsymbol{r}) \\ A\sin(\boldsymbol{q}\cdot\boldsymbol{r}) \\ B \end{pmatrix} . \tag{1}$$

Accordingly, the (non-interacting) Hamiltonian is given by (atomic units)

$$\begin{aligned} \hat{\mathcal{H}}_0 &= \int \mathrm{d}^3r \, \begin{pmatrix} \hat{\phi}^\dagger_\uparrow(\boldsymbol{r}) & \hat{\phi}^\dagger_\downarrow(\boldsymbol{r}) \end{pmatrix} \left(-\tfrac{1}{2}\nabla^2 - \mu - \tfrac{1}{2}\boldsymbol{B}(\boldsymbol{r})\cdot\boldsymbol{\sigma}\right) \begin{pmatrix} \hat{\phi}_\uparrow(\boldsymbol{r}) \\ \hat{\phi}_\downarrow(\boldsymbol{r}) \end{pmatrix} \\ &= \int \mathrm{d}^3r \, \begin{pmatrix} \hat{\phi}^\dagger_\uparrow(\boldsymbol{r}) & \hat{\phi}^\dagger_\downarrow(\boldsymbol{r}) \end{pmatrix} \begin{pmatrix} -\tfrac{1}{2}\nabla^2 - \mu - \tfrac{1}{2}B & -\tfrac{1}{2}Ae^{-\imath\boldsymbol{q}\cdot\boldsymbol{r}} \\ -\tfrac{1}{2}Ae^{\imath\boldsymbol{q}\cdot\boldsymbol{r}} & -\tfrac{1}{2}\nabla^2 - \mu + \tfrac{1}{2}B \end{pmatrix} \begin{pmatrix} \hat{\phi}_\uparrow(\boldsymbol{r}) \\ \hat{\phi}_\downarrow(\boldsymbol{r}) \end{pmatrix} . \end{aligned} \tag{2}$$

In momentum space the Hamiltonian can be written as,

$$\hat{\mathcal{H}}_0 = \int \mathrm{d}^3k \, \begin{pmatrix} \hat{\phi}^\dagger_\uparrow(\boldsymbol{k}-\tfrac{1}{2}\boldsymbol{q}) & \hat{\phi}^\dagger_\downarrow(\boldsymbol{k}+\tfrac{1}{2}\boldsymbol{q}) \end{pmatrix} \begin{pmatrix} -\tfrac{1}{2}\left(\boldsymbol{k}-\tfrac{1}{2}\boldsymbol{q}\right)^2 - \mu - \tfrac{1}{2}B & -\tfrac{1}{2}A \\ -\tfrac{1}{2}A & -\tfrac{1}{2}\left(\boldsymbol{k}+\tfrac{1}{2}\boldsymbol{q}\right)^2 - \mu + \tfrac{1}{2}B \end{pmatrix} \begin{pmatrix} \hat{\phi}_\uparrow(\boldsymbol{k}-\tfrac{1}{2}\boldsymbol{q}) \\ \hat{\phi}_\downarrow(\boldsymbol{k}+\tfrac{1}{2}\boldsymbol{q}) \end{pmatrix} . \tag{3}$$

The Hamiltonian matrix can be diagonalized yielding

$$\hat{\mathcal{H}}_0 = \int \mathrm{d}^3k \, \begin{pmatrix} \hat{\xi}^\dagger_-(\boldsymbol{k}) & \hat{\xi}^\dagger_+(\boldsymbol{k}) \end{pmatrix} \begin{pmatrix} \epsilon_-(\boldsymbol{k}) - \mu & 0 \\ 0 & \epsilon_+(\boldsymbol{k}) - \mu \end{pmatrix} \begin{pmatrix} \hat{\xi}_-(\boldsymbol{k}) \\ \hat{\xi}_+(\boldsymbol{k}) \end{pmatrix} , \tag{4}$$

where the operators $\hat{\xi}_-(\boldsymbol{k})$ and $\hat{\xi}_+(\boldsymbol{k})$ represent the so-called spin-spiral-wave orbitals [1, 2]

$$\xi_{\boldsymbol{k},-}(\boldsymbol{r}) = \begin{pmatrix} \cos\left(\tfrac{1}{2}\theta(\boldsymbol{k})\right) e^{-\frac{\imath}{2}\boldsymbol{q}\cdot\boldsymbol{r}} \\ \sin\left(\tfrac{1}{2}\theta(\boldsymbol{k})\right) e^{\frac{\imath}{2}\boldsymbol{q}\cdot\boldsymbol{r}} \end{pmatrix} \frac{e^{i\boldsymbol{k}\cdot\boldsymbol{r}}}{\sqrt{2\pi}^3} , \tag{5a}$$

$$\xi_{\boldsymbol{k},+}(\boldsymbol{r}) = \begin{pmatrix} -\sin\left(\tfrac{1}{2}\theta(\boldsymbol{k})\right) e^{-\frac{\imath}{2}\boldsymbol{q}\cdot\boldsymbol{r}} \\ \cos\left(\tfrac{1}{2}\theta(\boldsymbol{k})\right) e^{\frac{\imath}{2}\boldsymbol{q}\cdot\boldsymbol{r}} \end{pmatrix} \frac{e^{i\boldsymbol{k}\cdot\boldsymbol{r}}}{\sqrt{2\pi}^3} , \tag{5b}$$

and the corresponding orbital energies are

$$\epsilon_\mp(\boldsymbol{k}) = \tfrac{1}{2}k^2 + \tfrac{1}{8}q^2 \mp \tfrac{1}{2}\sqrt{\left(\boldsymbol{q}\cdot\boldsymbol{k} + B\right)^2 + A^2} . \tag{6}$$

The spin magnetization can be calculated from the orbitals, i.e. ,

$$\boldsymbol{m}(\boldsymbol{r}) = \int \mathrm{d}^3k \, \left\{ f_{(\epsilon_-(\boldsymbol{k})-\mu)} \xi^\dagger_{\boldsymbol{k},-}(\boldsymbol{r})\,\boldsymbol{\sigma}\xi_{\boldsymbol{k},-}(\boldsymbol{r}) + f_{(\epsilon_+(\boldsymbol{k})-\mu)} \xi^\dagger_{\boldsymbol{k},+}(\boldsymbol{r})\,\boldsymbol{\sigma}\xi_{\boldsymbol{k},+}(\boldsymbol{r}) \right\} = \begin{pmatrix} a\cos(\boldsymbol{q}\cdot\boldsymbol{r}) \\ a\sin(\boldsymbol{q}\cdot\boldsymbol{r}) \\ b \end{pmatrix} , \tag{7}$$

where $f_{(\epsilon)}$ is the Fermi distribution (step function at zero temperature). The amplitudes $a$ and $b$ are given by

$$a = -\frac{1}{(2\pi)^3}\int \mathrm{d}^3k \, \left(f_{(\epsilon_-(\boldsymbol{k})-\mu)} - f_{(\epsilon_+(\boldsymbol{k})-\mu)}\right) \frac{A}{\sqrt{(\boldsymbol{k}\cdot\boldsymbol{q}+B)^2 + A^2}} \, , \tag{8a}$$

$$b = -\frac{1}{(2\pi)^3}\int \mathrm{d}^3k \, \left(f_{(\epsilon_-(\boldsymbol{k})-\mu)} - f_{(\epsilon_+(\boldsymbol{k})-\mu)}\right) \frac{\boldsymbol{k}\cdot\boldsymbol{q}+B}{\sqrt{(\boldsymbol{k}\cdot\boldsymbol{q}+B)^2 + A^2}} \, , \tag{8b}$$

where we used the explicit form of the orbital rotation angle $\theta(\boldsymbol{k})$ appearing in the definitions (cf. Eq. (5)) of the spin-spiral-wave orbitals,

$$\cos(\theta(\boldsymbol{k})) = \frac{\boldsymbol{k}\cdot\boldsymbol{q}+B}{\sqrt{(\boldsymbol{k}\cdot\boldsymbol{q}+B)^2 + A^2}} \, , \tag{9a}$$

$$\sin(\theta(\boldsymbol{k})) = \frac{A}{\sqrt{(\boldsymbol{k}\cdot\boldsymbol{q}+B)^2 + A^2}} \, . \tag{9b}$$

This demonstrates that the external magnetic field Eq. (1) produces a spin magnetization of the form Eq. (7).

* feich@mpi-halle.mpg.de

[1] A. W. Overhauser, Phys. Rev. **128**, 1437 (1962).
[2] G. F. Giuliani and G. Vignale, "Spin density wave and charge density wave Hartree-Fock states," (Cambridge University Press, Cambridge, 2005) Chap. 2.6, pp. 90–101.
